# Supplementary material for: Analyzing Defense Strategies Against Mobile Information Leakages: A Game-Theoretic Approach
Source: arXiv:1904.13352 source file (2019-04-30)
Supplement: Supplementary file 1 [file appendix.tex]

\section*{Appendix}
